# Supplementary material for: How to Cooperate Locally to Improve Global Privacy in Social Networks? On Amplification of Privacy Preserving Data Aggregation
Source: arXiv:1704.05305 source file (2017-04-26)
Supplement: Supplementary file 1 [file appendix.tex]

\section*{Appendix}\label{sect:App}

apendiksy
